# Supplementary material for: Stable Blockchain Sharding under Adversarial Transaction Generation
Source: arXiv:2404.04438 source file (2024-04-19)
Supplement: Supplementary file 1 [file appendix.tex]

\section{Appendix}

\subsection{Example of Transaction processing}
\label{example-of-txn-processing}
\begin{example}
    Let's consider a scenario with four shards: $S_a$, $S_b$, $S_c$, and $S_d$, each holding a distinct account $a$, $b$, $c$, and $d$, respectively. The transactions are randomly assigned to shards, such that $S_a$ holds transaction $T_1$, $S_c$ holds transaction $T_2$ and $T_3$, and $S_d$ holds $T_4$ (i.e., home shard of each transaction). Moreover, transaction $T_1$ accesses accounts $a$ and $b$ in $S_a$ and $S_b$; $T_2$ accesses accounts $a$ and $d$ in $S_a$ and $S_d$; $T_3$ accesses accounts $b$ and $c$ in shard $S_b$ and $S_c$, and $T_4$ access accounts $c$ and $d$ in $S_c$ and $S_d$. The access pattern for each transaction is shown in Table \ref{tab:example}. We describe how basic distributed Algorithm \ref{alg:basic-distributed-scheduler} and fully distributed Algorithm \ref{alg:fully-distributed-scheduler} process these transactions.

    \begin{table}[!h]
      \caption{Transactions Information}
      \label{tab:example}
      \begin{tabular}{ccc}
        \toprule
        Txn (Home Shard) & Accessed Accounts (Destination Shard) & SubTxn \\
        \midrule
        $T_1 (S_a)$ & $a (S_a)$, $b (S_b)$ & $T_{1,a}, T_{1,b}$ \\
        $T_2 (S_c)$ & $a (S_a)$, $d (S_d)$ & $T_{2,a}, T_{2,d}$ \\
        $T_3 (S_c)$ & $b (S_b)$, $c (S_c)$ & $T_{3,b}, T_{3,c}$ \\
        $T_4 (S_d)$ & $c (S_c)$, $d (S_d)$ & $T_{4,c}, T_{4,d}$ \\
        \bottomrule
      \end{tabular}
    \end{table}

\end{example}

\paragraph{\bf Transaction Processing using Algorithm \ref{alg:basic-distributed-scheduler}}

The basic distributed scheduler model is depicted in Figure \ref{fig:centralized_model}, where we consider a uniform model and each shard is connected to every other shard with a distance of $1$ (i.e., they can exchange information within $1$ round). Assume that shard $S_a$ is the leader shard for the current epoch $E_i$, and all the transactions were generated in epoch $E_{i-1}$. Each shard knows the current leader shard $S_a$.

\begin{figure}[!ht]
\centering
\includegraphics[width=0.3\textwidth]{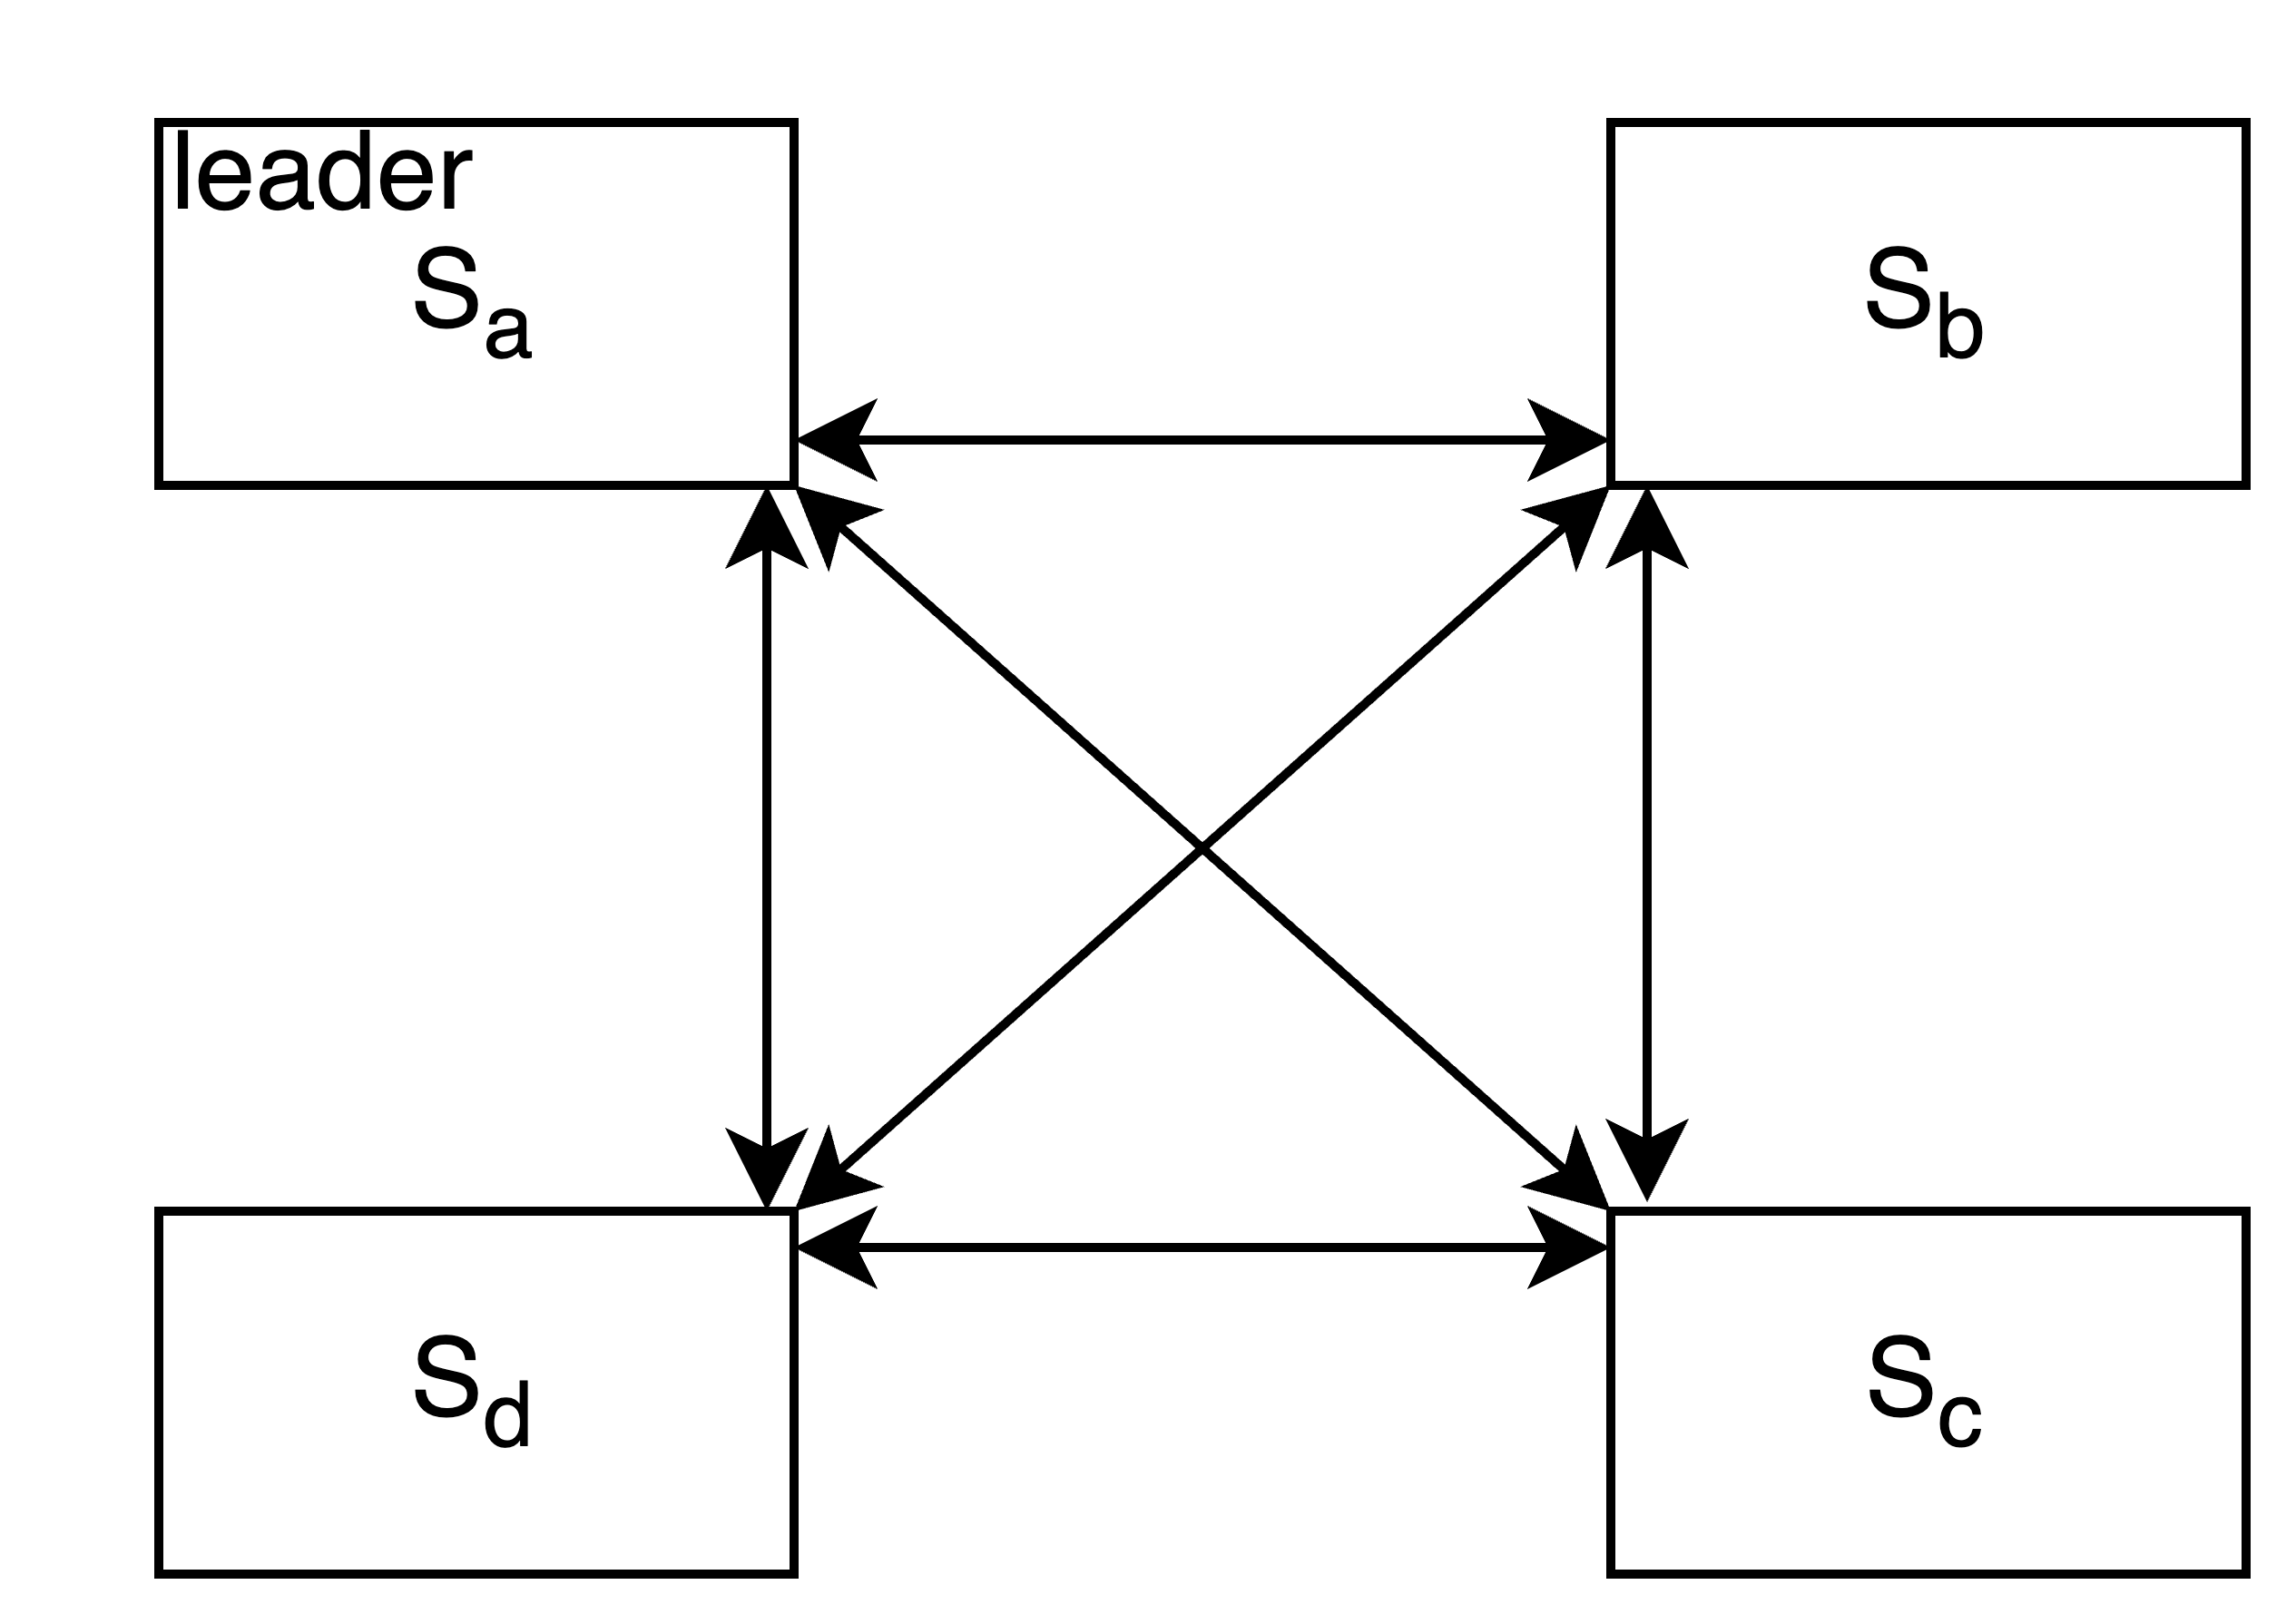}
\caption{Representation of the basic distributed scheduler model where shard $S_a$ is considered the leader.}
\label{fig:centralized_model}
\end{figure}

In the first phase of epoch $E_i$, all home shards with transactions in their pending queue send their transactions to the leader shard $S_a$. This phase takes only $1$ round, as all home shards can send their transactions in parallel.

In the second phase, $S_a$ creates a conflict graph of received transactions and colors that transaction graph to determine the schedule. Here, transactions $T_1$ and $T_4$ are non-conflicting, so they get the same color (let's say, color $0$). However, transactions $T_2$ and $T_3$ conflict with $T_1$, so they cannot receive color $0$. Consequently, the leader shard assigns color $1$ to transactions $T_2$ and $T_3$ (as $T_2$ and $T_3$ do not conflict with each other).
After the coloring process, $S_a$ sends the transaction color information back to the respective home shard ($S_a$, $S_c$, and $S_d$) of each transaction. This phase also takes $1$ round, assuming the shard has enough resources to color the transactions instantly.

In the third phase, each home shard schedules transactions based on the color they have been assigned. The maximum number of colors used to color all the transactions is $2$, so this phase takes $4 \times 2 = 8$ rounds to commit all transactions because each color takes $4$ rounds for confirmation and commit. For example, in the first round of Phase 3, the home shard of transactions $T_1$ and $T_4$ splits these transactions into subtransactions as $T_{1,a}, T_{1,b}$ and $T_{4,c}, T_{4,d}$ and sends them to the destination shards to check the condition of transaction In the second round, the destination shard checks the transaction condition and sends either a commit or abort vote. In the third round, leader shard $S_a$ collects all votes, and if it receives a commit vote, then it sends a confirm commit message to the respective destination shard, and if it receives any abort vote for a particular transaction, it sends a confirm abort vote. In round four, the destination shard either commits or aborts that subtransaction according to its received message. Similarly, transactions $T_2$ and $T_3$ are processed and committed in the next color round.

Thus, if the transaction was generated at round $t$, then the transactions are confirmed and committed at $t+6$, and their latency is $t+6$ rounds. Similarly,   transactions $T_2$ and $T_3$ are confirmed and committed at round $t+10$, and their latency is  $t+10$ rounds.

\paragraph{\bf Transaction Processing using Fully Decentralized Algorithm \ref{alg:fully-distributed-scheduler}}

In this fully decentralized model, we consider a non-uniform model where the distance between any two shards ranges from $1$ to $D$. Shards are organized into clusters, each belonging to one or more clusters. Within each cluster layer (sublayer), a designated leader is responsible for coloring and scheduling transactions. Figure \ref{fig:decentralized_model} shows a simplified representation of shard clustering.

Shards within a cluster layer $L1$—namely cluster $L1,SL1$, cluster $L1,SL2$, and cluster $L1,SL1'$—are at a maximum distance of $d_1$ from each other. Shards within cluster layer $L2$, specifically $L2,SL1$, are at a maximum distance of $d_2$ from each other. Additionally, shard $S_a$ serves as the leader for cluster $L1,SL1$, shard $S_b$ as the leader for cluster $L1,SL2$, shard $S_c$ as the leader for cluster $L1,SL1'$, and shard $S_d$ as the leader for cluster $L2,SL1$.

\begin{figure}[!ht]
\centering
\includegraphics[width=0.49\textwidth]{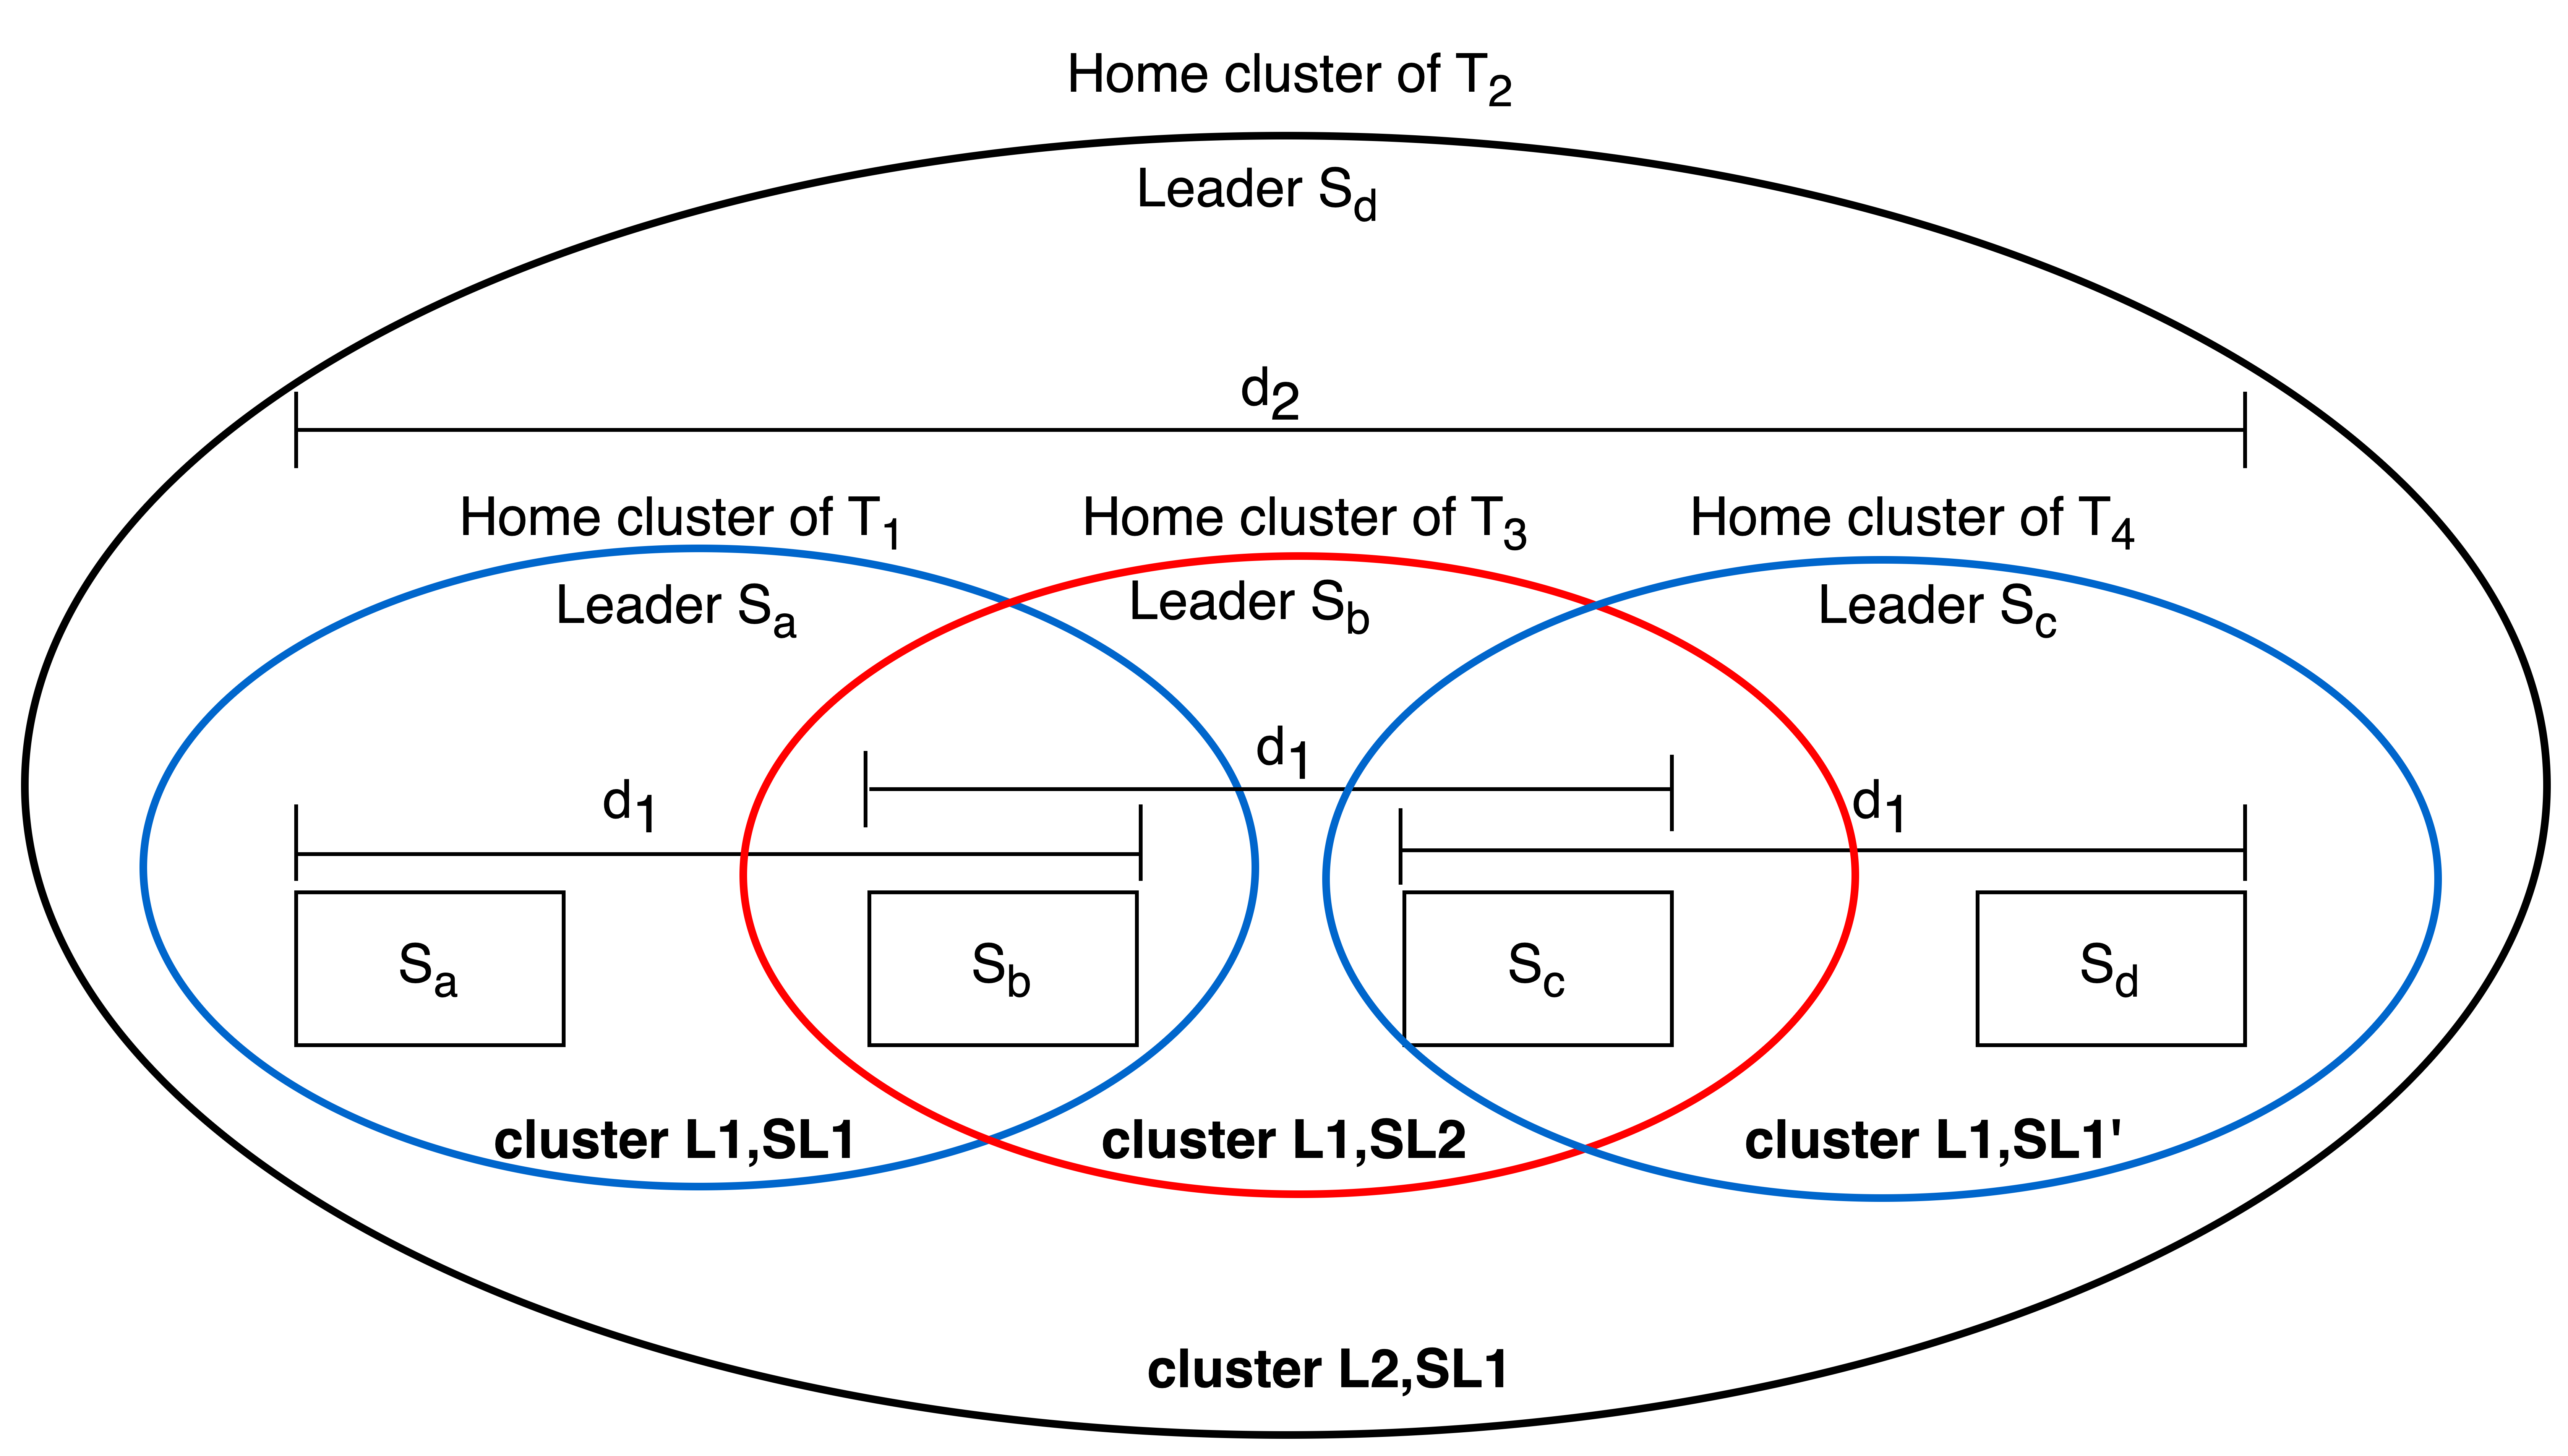}
\caption{Representation of the fully distributed model where each shard belongs to some cluster layers.}
\label{fig:decentralized_model}
\end{figure}

In our example, Transaction $T_1$ accesses shards $S_a$ and $S_b$, which are at a distance $d_1$ from each other and belong to the cluster $L_1,SL1$ (so we call cluster $L_1,SL1$ as the home cluster of $T_1$). The leader shard $S_a$ of that cluster determines the scheduling of $T_1$. Similarly, Transaction $T_2$ accesses shards $S_a$ and $S_d$, which are at a distance $d_2$ from each other and are part of cluster layer $L_2,SL1$ (i.e., the home cluster for $T_2$). The cluster leader shard ($S_d$) receives the transaction from the home shard of $T_2$ (i.e., $S_c$), colors the transactions, and determines the schedule.

Moreover, Transaction $T_3$ accesses shards $S_b$ and $S_c$, both of which are in cluster layer $L1,SL2$. So, the home shard of $T_3$ (i.e., $S_c$) labels the home cluster for Transaction $T_3$ as $L1SL2$, and $S_c$ sends the transactions to the cluster leader shard $S_b$, where $S_b$ colors the transactions and determines the schedule. Similarly, Transaction $T_4$ accesses shards $S_c$ and $S_d$, belonging to cluster $L_1,SL1'$. The home shard (i.e., $S_d$) of $T_4$ sends the transaction to the leader shard (i.e., $S_c$) of the home cluster of $T_4$. In this case, the leader shard $S_c$, handles the transactions, so $S_d$ sends (moves) its transaction to $S_c$ for coloring and scheduling.

Suppose the epoch length of layer $L_1$ is $x_{d_1}$, and the epoch length of layer $L_2$ is $x_{d_2}$ (which is a multiple of $L_1$). The beginning of the epoch is the same for all layers. However, transactions that belong to layer $L_1$ can propagate from their home shard to cluster leader shard within $d_1$ rounds, but transactions belonging to layer $L_2$ take $d_2$ rounds (where $d_1<d_2$). So in the first $d_1$ rounds, the home shard of transaction $T_1$, $T_3$, and $T_4$ sends these transactions to respective cluster leader shards. After that, the cluster leader shard colors the received transactions splits colored transactions and sends them to the destination shard, which takes another $d_1$ rounds. So transactions $T_1$, $T_3$, and $T_4$ are scheduled in destination shard at $2d_1$ rounds. Similarly, transacitons $T_2$ are scheduled in destination shard at $2d_2$ rounds.

% After coloring the transactions, each cluster leader splits the colored transactions into subtransactions and sends them to the destination shards, where the destination shards decide which subtransaction needs to be processed first.

Thus, transactions $T_1$, $T_3$ and $T_4$ are gets scheduled at round $t+2d_1$ and transactions $T_2$ get scheduled at $t+2d_2$.

Each destination shard maintains a scheduled queue, organizing received subtransactions in lexicographic order based on epoch end, layer, sublayer, and color.
For example, Transaction $T_1$ takes an additional $3d_1$ round to get confirmed and committed because the cluster leader shard and destination shard need to communicate back and forth to confirm and commit the transaction. Thus, transaction $T_1$ gets committed within $t+2d_1+3d_1= t+5d_1$ rounds, while Transaction $T_2$ takes $t+5d_2$ rounds to commit (i.e., the time to commit Transaction $T_1$ is less than $T_2$).

Similarly, in destination shards $S_b$ and $S_c$, subtransactions $T_{1,b}, T_{3,b}$ and $T_{3,c}, T_{4,c}$ gets priority for processing according to their epoch end, sublayer, and color, as they belong to the same layer $L1$. Moreover, in destination shard $S_d$, subtransaction $T_{4,d}$ gets priority to commit, as it received the subtransaction from cluster $L1,SL'$ with a maximum cluster distance of $d_1$, followed by subtransaction $T_{2,d}$. This priority and order remain consistent in each destination shard according to the lexicographic we defined in the algorithm. Thus, there will be no deadlock situation.
